# Supplementary material for: A solid-state temporally multiplexed quantum memory array at the single-photon level
Source: arXiv:2507.12200 source file (2025-07-16)
Supplement: Supplementary file 1 [file supplementary.pdf]

# Supplementary: A solid-state temporally multiplexed quantum memory array at the single-photon level

Markus Teller[1*†], Susana Plascencia[1†], Cristina Sastre Jachimska[1], Samuele Grandi[1], Hugues de Riedmatten[1,2]

[1]ICFO-Institut de Ciencies Fotoniques, The Barcelona Institute of Science and Technology, Castelldefels (Barcelona), 08860, Spain.
[2]ICREA, Institucio Catalana de Recerca i Estudis Avançats, Barcelona, 08015, Spain.

*Corresponding author(s). E-mail(s): markus.teller@icfo.eu;
†These authors contributed equally to this work.

## 1 Setup efficiencies

In Fig. 1, we provide a complete list of efficiencies of the experimental setup per spatial mode. Details of each element are provided in the main text.

| | 1 | 2 | 3 | 4 | 5 | 6 | 7 | 8 | 9 | 10 |
|---|---|---|---|---|---|---|---|---|---|---|
| Multiplex $\eta_{\mathrm{m}}$ | 90.5(4) | 90.9(3) | 91.2(3) | 89.9(6) | 90.0(3) | 88.1(3) | 88.3(4) | 86.7(4) | 86.0(4) | 86.1(3) |
| AFC $\tau = 10\ \mu$s | 17.8(7) | 19.1(6) | 18.0(8) | 17(1) | 17(1) | 16.2(7) | 16(1) | 15.7(8) | 14(1) | 13.4(6) |
| AFC $\tau = 25\ \mu$s | 6.4(5) | 7.9(4) | 7.0(9) | 7(1) | 5.6(9) | 4.9(5) | 5.4(6) | 4.6(8) | 4.7(4) | 4.0(3) |
| Two-Way Transfer | 20(1) | 23(1) | 28(2) | 28(2) | 32(2) | 33(3) | 36(4) | 32(3) | 27(3) | 33(5) |
| Demultiplex $\eta_{\mathrm{d}}$ | 65(3) | 73(4) | 81(5) | 90(8) | 92(8) | 89(6) | 90(8) | 83(7) | 76(8) | 68(6) |
| Fiber | 26(2) | 33(1) | 42(2) | 49(3) | 57(3) | 58(3) | 57(3) | 51(3) | 45(4) | 29(2) |
| SW Memory $\tau = 10\ \mu$s | 3.5(1) | 4.4(1) | 5.0(2) | 4.8(4) | 5.4(4) | 5.3(2) | 5.7(4) | 5.0(3) | 4.0(3) | 4.5(2) |
| SW Memory $\tau = 25\ \mu$s | 1.3(1) | 1.8(1) | 1.9(1) | 2.0(2) | 1.8(2) | 1.6(2) | 2.0(2) | 1.4(2) | 1.3(2) | 1.3(2) |
| Total $\tau = 10\ \mu$s | 0.53(6) | 0.95(9) | 1.6(2) | 1.9(3) | 2.6(4) | 2.4(3) | 2.6(4) | 1.9(3) | 1.2(2) | 0.8(2) |
| Total $\tau = 25\ \mu$s | 0.19(3) | 0.40(4) | 0.6(1) | 0.8(2) | 0.8(2) | 0.7(1) | 0.9(2) | 0.5(1) | 0.4(1) | 0.23(5) |

Mode

**Fig. 1** Complete list of efficiencies of the experimental setup obtained with classical light and provided in percent.
